# Supplementary material for: Protenix-Mini+: efficient structure prediction model with scalable pairformer
Source: arXiv:2510.12842 source file (2025-10-16)
Supplement: Supplementary file 1 [file appendix.tex]

\section{Hello World}
%\subsection{Hello World}
